# Supplementary material for: Enhancing Contention Resolution ALOHA using Combining Techniques
Source: arXiv:1602.07636 source file (2017-10-06)
Supplement: Supplementary file 1 [file Appendix.tex]

\section*{Appendix - Probability of loops}
